# Supplementary material for: Density Functional Theory of the Hubbard-Holstein Model
Source: arXiv:1903.04984 ancillary file (2019-03-12)
Supplement: Supplementary file 1 [file SupplementalHHsubmit.pdf]

# Density Functional Theory of the Hubbard-Holstein Model (Supplemental Material)

E. Viñas Boström,[1] P. Helmer,[1] P. Werner,[2] and C. Verdozzi[1]

[1] *Department of Physics and ETSF, Lund University, PO Box 118, 221 00 Lund, Sweden*
[2] *Department of Physics, University of Fribourg, 1700 Fribourg, Switzerland*

(Dated: March 12, 2019)

## THE MODEL

The Hamiltonian of the inhomogeneous Hubbard-Holstein model is given by

$$H = \sum_{i\sigma} (v_i - \mu)\hat{n}_{i\sigma} + U \sum_i \hat{n}_{i\uparrow}\hat{n}_{i\downarrow} - J \sum_{\langle ij \rangle \sigma} c^\dagger_{i\sigma} c_{j\sigma} + \omega \sum_i b^\dagger_i b_i + \sum_i \sqrt{2}\eta_i \, \hat{x}_i + \sqrt{2} g \sum_i (\hat{n}_i - 1)\hat{x}_i, \tag{1}$$

where $\hat{n}_i = \hat{n}_{i\uparrow} + \hat{n}_{i\downarrow}$. In Eq. (1), $v_i$ and $\eta_i$ are taken as site dependent, which is convenient to address basic aspects of the (TD)DFT formulation. However, later on we specialize to site-independent potentials, and solve for the homogeneous reference HH lattice, needed to devise and use an (adiabatic) local density approximation.

## HOHENBERG-KOHN THEOREM FOR THE GROUND STATE OF THE HH MODEL

We next establish the Hohenberg-Kohn theorem for electron-phonon systems, by proving the existence of a bijective map between the pairs of conjugate variables $(\mu, \eta)$ and $(n, x)$. The proof is based on the constrained variational method introduced by Levý [1], and closely follows the line of reasoning of Schönhammer, Gunnarsson and Noack [2]. However, a proof following directly the logic of the original HK formulation is also possible [3].

We construct a Kohn-Sham system of non-interacting electrons and phonons, which for $v$- and $\eta$-representable systems follows from the variational property of the total energy. We assume the Hamiltonian to be of the form

$$H = H_0 + \sum_i v_i \hat{n}_i + \sqrt{2} \sum_j \eta_j \hat{x}_j, \tag{2}$$

where $\mu$ is an external potential acting on the electrons, and $\eta$ is a corresponding phonon potential. In the case of the Hubbard-Holstein model, we have

$$H_0 = -\mu \sum_{i\sigma} \hat{n}_{i\sigma} + U \sum_i \hat{n}_{i\uparrow}\hat{n}_{i\downarrow} - J \sum_{\langle ij \rangle \sigma} \left( c^\dagger_{i\sigma} c_{j\sigma} + h.c. \right) + \omega \sum_i b^\dagger_i b_i + \sqrt{2} g \sum_i (\hat{n}_i - 1)\hat{x}_i, \tag{3}$$

The theorem we want to prove is the following:

**Theorem (Hohenberg-Kohn).** *For given $\{v_i\}$ and $\{\eta_j\}$, let $|\Psi_0\rangle$ be the ground state of the Hamiltonian in Eq. (2) with energy $E_0$. For any state $|\Phi\rangle$, define the energy by $E = \langle \Phi | H | \Phi \rangle$, the local electron density by $n_i = \langle \Phi | \hat{n}_i | \Phi \rangle$ and the mean phonon coordinate by $x_j = \langle \Phi | \hat{x}_j | \Phi \rangle$. Then the total energy $E$ of the system is a functional of the local electron densities $n_i$ and phonon coordinates $x_j$ and satisfies the variational property $E(\{n_i, x_i\}) \geq E_0$, with equality if and only if the densities and coordinates are given by their ground state values.*

*Proof.* We define $M(\{n_i\}, \{x_j\})$ as the set of wavefunctions $|\Phi(\{n_i\}, \{x_j\})\rangle$ that give the specific set of eigenvalues $\{n_i\}$ and $\{x_j\}$. Further, we define $F(\{n_i\}, \{x_i\})$ as the smallest value in the set $M$, so that

$$F(\{n_i\}, \{x_i\}) = \min_{|\phi\rangle \in M} \langle \phi | H_0 | \phi \rangle . \tag{4}$$

The total energy of the system is then given by

$$E(\{n_i\}, \{x_i\}) = F(\{n_i\}, \{x_i\}) + \sum_i v_i \hat{n}_i + \sqrt{2} \sum_j \eta_j x_j. \tag{5}$$

If we pick a state $|\Phi\rangle \in M$ such that $H_0$ attains its minimal value $F(\{n_i\},\{x_i\})$, we find

$$\begin{aligned} E(\{n_i, x_i\}) &= \langle\Phi| H_0 |\Phi\rangle + \sum_i v_i n_i + \sqrt{2}\sum_j \eta_j x_j \\ &= F(\{n_i, x_i\}) + \sum_i v_i n_i + \sqrt{2}\sum_j \eta_j x_j \geq E_0, \end{aligned} \tag{6}$$

where $E_0$ is the ground state energy of $H$. This follows directly from the variational principle stating that any wavefunction $|\Phi\rangle$ will give an energy that is larger than or equal to the ground state energy of the system. We then pick another wavefunction $|\Psi\rangle$, which produces the ground state energy $E_0$. In other words, $|\Psi\rangle$ is a ground state of the system described by $H$. We denote by $n_i^0 = \langle\Psi| \hat{n}_i |\Psi\rangle$ and $x_i^0 = \langle\Psi| \hat{x}_i |\Psi\rangle$ the ground state values of the density and position. Then we obtain

$$\begin{aligned} E_0 = \langle\Psi| H |\Psi\rangle &= \langle\Psi| H_0 |\Psi\rangle + \sum_i v_i n_i^0 + \sqrt{2}\sum_j \eta_j x_j^0 \\ &\geq F(\{n_i^0, x_i^0\}) + \sum_i v_i n_i^0 + \sqrt{2}\sum_j \eta_j x_j^0 = E(\{n_i^0, x_i^0\}). \end{aligned} \tag{7}$$

This follows from the fact that although $|\Psi\rangle \in M[n^0, x^0]$, it may not be the state for which $F(\{n_i^0, x_i^0\})$ is attained. Hence we have obtained two inequalities $E(\{n_i, x_i\}) \geq E_0$ and $E(\{n_i^0, x_i^0\}) \leq E_0$, but since the first inequality holds for all $\{n_i.x_i\}$ this in particular implies

$$E(\{n_i, x_i\}) \geq E(\{n_i^0, x_i^0\}) = E_0. \tag{8}$$

With this we have shown that the total energy $E(\{n_i, x_i\})$ is a functional of $n$ and $x$ that, for given $v$ and $\eta$, is minimized for the correct ground state values $n^0$ and $x^0$. Furthermore, for a non-degenerate ground state the density $n^0$ and displacement $x^0$ are completely determined by minimizing the total energy $E$.

□

This completes our discussion of the ground state of the HH model. To provide firm conceptual ground to a time-dependent treatment, a proof originally given for a TDDFT of electron-photon lattice systems [8] (with electron densities and photon momenta as fundamental variables) should be adapted to the present case with $n$ and $x$ as basic variables.

## KOHN-SHAM SYSTEM

We now derive a set of coupled independent particle equations for the electrons and phonons respectively, that give the same ground state expectation values $n^0$ and $x^0$ as the coupled system. Since the total energy satisfies the variational principle with respect to $n$ and $x$, and the ground state energy is a global minimum, the functional derivatives with respect to the variables $n$ and $x$ are both zero in the ground state. This gives the two sets of Euler equations

$$\begin{aligned} \frac{\delta F}{\delta n_i} + v_i &= 0, \\ \frac{\delta F}{\delta x_j} + \sqrt{2}\eta_j &= 0, \end{aligned} \tag{9}$$

with $F(\{n_i\},\{x_i\})$ defined as above. To simplify the notation we will use $n = \{n_i\}$ and $x = \{x_j\}$ to denote the full set of electronic densities and phononic displacements. We decompose the total energy $E[n, x]$ according to

$$E[n, x] = T_e^0[n] + T_{ph}^0[x] + E_{ext}^e[n] + E_{ext}^{ph}[x] + E_H^e[n] + E_H^{e-ph}[n, x] + E_{xc}[n, x], \tag{10}$$

in order to separate the interaction energy from the non-interacting contributions. Here the first two terms $T_e^0$ and $T_{ph}^0$ give the kinetic energy of the noninteracting electron and phonon system, respectively, the next two terms $E_{ext}^e$ and $E_{ext}^{ph}$ the energies from the external potentials, followed by the Hartree energies $E_H^e$ and $E_H^{e-ph}$ of the electron-electron

and electron-phonon interaction. The last term is the exchange-correlation (xc) energy, containing everything left out by the other terms. Taking the variation of the total energy yields

$$\begin{aligned}
\delta E &= \sum_i \frac{\delta E[n,x]}{\delta n_i}\delta n_i + \sum_j \frac{\delta E[n,x]}{\delta x_j}\delta x_j \qquad (11)\\
&= \sum_i \delta n_i \left( \frac{\delta T_e^0[n]}{\delta n_i} + \frac{\delta E_{ext}^e[n]}{\delta n_i} + \frac{\delta E_H[n]}{\delta n_i} + \frac{\delta E_H^{e-ph}[n,x]}{\delta n_i} + \frac{\delta E_{xc}[n,x]}{\delta n_i} \right)\\
&+ \sum_j \delta x_j \left( \frac{\delta T_{ph}^0[x]}{\delta x_j} + \frac{\delta E_{ext}^{ph}[x]}{\delta x_j} + \frac{\delta E_H^{e-ph}[n,x]}{\delta x_j} + \frac{\delta E_{xc}[n,x]}{\delta x_j} \right)\\
&= \sum_i \delta n_i \left( \frac{\delta T_e^0[n]}{\delta n_i} + v_i^{ext}[n] + v_{i,e}^H[n] + v_{i,e-ph}^H[x] + v_i^{xc}[n,x] \right)\\
&+ \sum_j \delta x_j \left( \frac{\delta T_{ph}^0[x]}{\delta x_j} + \sqrt{2}\eta_j^{ext}[x] + \sqrt{2}\eta_{j,e-ph}^H[n] + \sqrt{2}\eta_j^{xc}[n,x] \right),
\end{aligned}$$

where in the last line we have introduced the notation $v_e^H$, $v_{e-ph}^H$ and $\eta_{e-ph}^H$ for the Hartree potentials of the electron-electron and electron-phonon interaction. Demanding that $\delta E = 0$ for arbitrary variations $\delta n$ and $\delta x$, this gives the equations of motion of the system.

We now recognize that the above expression can also be obtained from the Euler equations in Eq. (9) if we take the Hamiltonian to be

$$\begin{aligned}
H_{KS} &= -\mu \sum_{i\sigma} \hat{n}_{i\sigma} - J \sum_{\langle ij\rangle\sigma} \left( c_{i\sigma}^\dagger c_{j\sigma} + h.c. \right) + \sum_{i\sigma} v_i^{KS}[n,x]\hat{n}_{i\sigma} + \omega \sum_j b_j^\dagger b_j + \sqrt{2}\sum_j \eta_j^{KS}[n,x]\hat{x}_j\\
&= H_0 + \sum_{i\sigma} v_i^{KS}[n,x]\hat{n}_{i\sigma} + \sqrt{2}\sum_j \eta_j^{KS}[n,x]\hat{x}_j, \qquad (12)
\end{aligned}$$

where the Kohn-Sham potentials are $v_i^{KS} = v_i^{ext} + v_{i,e}^H + v_{i,e-ph}^H + v_i^{xc}$ and $\eta_j^{KS} = \eta_j^{ext} + \eta_{j,e-ph}^H + \eta_j^{xc}$. These equations need to be solved with the additional restriction that the ground state of $\hat{H}_{KS}$ reproduces the correct ground state electron density and phonon displacement. This leads to the coupled pair of Kohn-Sham equations

$$\hat{H}_{KS}^e |\psi_m^e\rangle = \left( -t \sum_{\langle ij\rangle\sigma} \left( c_{i\sigma}^\dagger c_{j\sigma} + h.c \right) + \sum_{i\sigma} v_i^{KS}[n,x]\hat{n}_{i\sigma} \right) |\psi_m^e\rangle = \varepsilon_m^e |\psi_m^e\rangle, \qquad (13)$$

$$\hat{H}_{KS}^{ph} |\chi_n^{ph}\rangle = \sum_j \left( \omega b_j^\dagger b_j + \sqrt{2}\eta_j^{KS}[n,x]\hat{x}_j \right) |\chi_n^{ph}\rangle = \varepsilon_n^{ph} |\chi_n^{ph}\rangle. \qquad (14)$$

## TOTAL ENERGY OF THE HOMOGENEOUS SYSTEM AND USE OF THE LANG-FIRSOV TRANSFORMATION

To compute the total energy of the reference system, we consider the homogeneous version of the system, where the expectation values of all local observables are independent of the site index. In particular, this means $v_i = v$ and $\eta_j = \eta$ so that we can write $x_i = x$ and $n_i = n$. To simplify the numerical evaluation of the ground state energy, the electron-phonon interaction can be decoupled using the Lang-Firsov transformation $H' = e^{iS} H e^{-iS}$, where

$$S = \frac{\sqrt{2}}{\omega} \sum_i \left[ g(\hat{n}_i - 1) + \eta \right] \hat{p}_i, \qquad (15)$$

and $\hat{p}_i = i(b_i^\dagger - b_i)/\sqrt{2}$ is the phonon momentum. Using the Baker-Hausdorff formula to perform the manipulations we find the transformed Hamiltonian

$$H' = \sum_{i\sigma} (v' - \mu)\hat{n}_{i\sigma} + \sum_i U' \hat{n}_{i\uparrow}\hat{n}_{i\downarrow} - \sum_{\langle ij\rangle\sigma} \left( \hat{t}_{ij}' c_{i\sigma}^\dagger c_{j\sigma} + h.c. \right) + \sum_i \left[ \omega b_i^\dagger b_i - \frac{(\eta - g)^2}{\omega} \right], \qquad (16)$$

where the parameters are given by $v' = v + (g^2 - 2g\eta)/\omega$, $U' = U - 2g^2/\omega$ and $\hat{t}'_{ij} = te^{i\sqrt{2}g(\hat{p}_i - \hat{p}_j)/\omega}$. We note that the hopping amplitude is now an operator which acts on the phonon states.

To construct the exchange-correlation potentials, we need to evaluate the ground state energy of the Hubbard-Holstein model for all $n$ and $x$. For given values of the interaction $U$, electron-phonon coupling $g$ and phonon frequency $\omega$, this in principle means that we need to solve the model for all values of $v$, $\mu$ and $\eta$. The calculation is however simplified by noting that the transformed Hamiltonian $H'$, Eq.(16), depends only on the effective parameter $-\mu' = v' - \mu = v + (g^2 - 2g\eta)/\omega - \mu$ (up to an $\eta$-dependent constant). In addition, for a homogeneous system $v$ is a redundant variable that can be set to zero by a suitable redefinition of the chemical potential. Although in principle $\mu'$ still depends on $\eta$, in practice we treat $\mu'$ as an independent parameter.

To determine the ground state energy $E_0[\mu, \eta]$, it suffices to find its value for all $\mu'$ and $\eta = 0$. The energy in the general case can then be obtained from the case where $\eta = 0$ through the relation

$$E_0[\mu, \eta] = E_0[\mu'(\mu, \eta)] - \frac{(\eta - g)^2}{\omega}. \tag{17}$$

Since in the end we want the energy as a function of the density $n$ and position $x$, we need to relate their values for general $\mu$ and $\eta$ to the case where $\eta = 0$. However, it follows from the Heisenberg equation of motion for the phonon momentum, $\partial_t p = i\hbar^{-1}[H, p] = 0$, that $x = -\sqrt{2}\,[g(n-1) + \eta]\,/\omega$. This means that the phonon coordinate $x$ is completely determined by $n$ and $\eta$. To obtain the energy as a function of $n$ and $x$ it is therefore sufficient to calculate $E_0$ and $n$ as a function of $\mu'$ (for $\eta = 0$), which allows to determine $n$ as a function of $\mu'$. We can then determine $E_0$ for all values of $\eta$, and finally invert the relation above to obtain $x$ as a function of $n$ and $\eta$. This completely determines $E_0[n, x]$, as shown in more detail below.

**Explicit expressions for $E$ and $E_{xc}$**

We write the total energy as the sum of terms in Eq. (16), using the explicit expressions for $\mu'$ and $\eta$,

$$\begin{aligned} \mu' &= \mu - \frac{g^2}{\omega} + \frac{2g\eta}{\omega}, \\ \eta &= -g(n-1) - \frac{\omega x}{\sqrt{2}}, \end{aligned} \tag{18}$$

to eliminate these variables. The term proportional to $\mu'$ is given by

$$-\mu' n_i = -\left(\mu - \frac{g^2}{\omega} + \frac{2g\eta}{\omega}\right) n_i = -\mu n_i + \frac{g^2 n_i}{\omega} + \sqrt{2} g n_i x_i + \frac{2g^2 n_i}{\omega}(n_i - 1),$$

while the constant term can be expanded as

$$-\frac{(\eta - g)^2}{\omega} = -\frac{\omega x_i^2}{2} - \frac{g^2 n_i^2}{\omega} - \sqrt{2} g n_i x_i. \tag{19}$$

For the total energy we then find the expression

$$\begin{aligned} E &= T[n] + \sum_i \left[ U' \langle n_{i\uparrow} n_{i\downarrow} \rangle + \omega n_{i,ph} - \mu n_i + \frac{g^2 n_i}{\omega} + \sqrt{2} g n_i x_i + \frac{2g^2 n_i}{\omega}(n_i - 1) - \frac{\omega x_i^2}{2} - \frac{g^2 n_i^2}{\omega} - \sqrt{2} g n_i x_i \right] \\ &= T[n] + \sum_i \left[ U' \langle n_{i\uparrow} n_{i\downarrow} \rangle + \omega n_{i,ph} - \mu n_i + \frac{g^2 n_i}{\omega}(n_i - 1) - \frac{\omega x_i^2}{2} \right], \end{aligned} \tag{20}$$

where $T[n] = -J \sum_{\langle ij \rangle \sigma} \langle c^\dagger_{i\sigma} c_{j\sigma} \rangle$ is the kinetic energy of the electrons. To obtain the exchange-correlation energy $E_{xc}$, we write it in the form

$$E_{xc} = E - E^e_{ext} - E^{ph}_{ext} - E^{e-e}_H - E^{e-ph}_H - E^e_0 - E^{ph}_0. \tag{21}$$

The external energies are given respectively by $E^e_{ext} = -\mu \sum_i n_i$ and $E^{ph}_{ext} = \sqrt{2}\eta \sum_i x_i = -\sum_i [\omega x_i^2 + \sqrt{2} g x_i (n_i - 1)]$, while the Hartree contributions from the electron-electron and electron-phonon interactions are $E^{e-e}_H = (U/4) \sum_i n_i^2$ and $E^{e-ph}_H = \sqrt{2} g \sum_i x_i (n_i - 1)$. For the phonons we find the non-interacting energy

$$E^{ph}_0 = \sum_i \left[ \omega n_{i,ph} - \frac{\eta_0^2}{\omega} - \sqrt{2}\eta_0 x_i \right] = \frac{\omega}{2} \sum_i x_i^2, \tag{22}$$

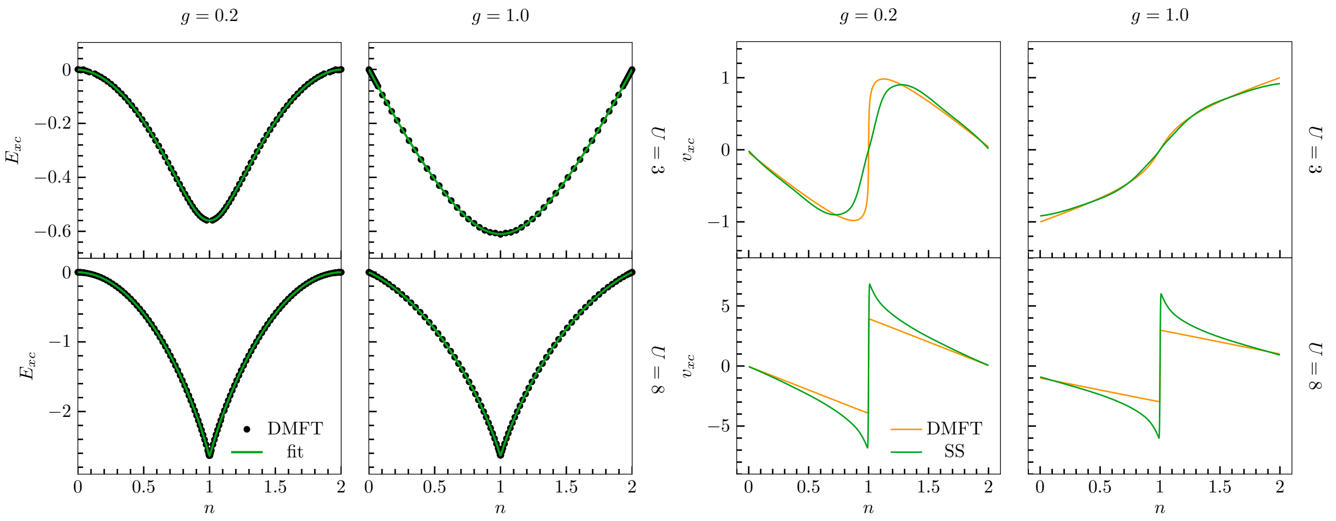


FIG. 1: Exchange-correlation energy $E_{xc}$ and exchange-correlation potential $v_{xc}$ as a function of electron density $n$, for different values of the electron-electron interaction $U$ and electron-phonon interaction $g$. In all figures $\omega = 1$ and $x = 0$, which gives $\eta = -g(n-1)$. The black dots are the DMFT numerical data and the green curves the numerical fit. The same applies to the $v_{xc}$ panels where, for comparison, the single site results (orange curves) are also reported (see main text).

where we have used that for a non-interacting system $x_i = -\sqrt{2}\eta_0/\omega$. Denoting the kinetic energy of the non-interacting electron system by $T_0[n] = -J\sum_{\langle ij\rangle\sigma}\langle c^\dagger_{i\sigma}c_{j\sigma}\rangle_0$ (taken over the noninteracting ground state), we obtain the exchange-correlation energy

$$E_{xc} = T[n] - T_0[n] + \sum_i \left[U'\langle n_{i\uparrow}n_{i\downarrow}\rangle + \omega n_{i,ph} - U\frac{n_i^2}{4} + \frac{g^2 n_i}{\omega}(n_i - 1)\right]. \tag{23}$$

We used dynamical mean-field theory (DMFT) to calculate the total energy $E$, and constructed the exchange-correlation energy from the expression above. In practice this was done by measuring the observables in Eq. (23) with DMFT, namely the kinetic energy, the double occupancy, the electron density and the phonon density. The hybridization expansion continuous-time Monte Carlo approach [6] allows to obtain the kinetic energy from the average perturbation order, and the density and double occupation from the average length and overlap of the spin-up and spin-down segments. To measure the phonon occupation, we insert the operator $O = e^{xb^\dagger - yb}$ at imaginary time $\tau = 0$ and calculate the corresponding Monte Carlo weights following Ref. 7. Taking appropriate derivatives with respect to $x$ and $y$ and setting $x = y = 0$ leads to the measurement formula for $n_{ph}$.

The resulting $E_{xc}$ as a function of $n$ is shown in Fig. 1 for different values of $U$ and $g$, taking $\omega = 1$ and $x = 0$. The DMFT data for the XC energy were fitted using piecewise polynomials of fourth order for $n$ in the interval $[0, 1]$, to obtain a function $E_{xc}(n)$. The exchange-correlation potential was then found from the derivative $v_{xc}(n) = \partial E_{xc}(n)/\partial n$ and is also shown in Fig. 1.

## SPECTRAL FUNCTION

The thermal spectral function $A(\epsilon)$ can be calculated by evaluating the Matsubara Greens function $G^M(\tau) = (iZ)^{-1}\mathrm{Tr}\left(e^{-\beta H}\mathcal{T}[c(\tau)c^\dagger(0)]\right)$, and later Fourier transforming to energy. Since in the Fourier transform of $G^M$ we can restrict to $\tau > 0$, we need only evaluate this part of $G^M$. For a single Hubbard-Holstein site one obtains

$$\begin{aligned} G^M(\tau) &= (iZ)^{-1}\sum_{\alpha\sigma m}\langle\alpha m|e^{-\beta H^M}c_\sigma(\tau)c^\dagger_\sigma(0)|\alpha m\rangle \qquad (24)\\ &= 2(iZ)^{-1}\sum_m\left[e^{\tau(\mu-v)}\langle m|e^{(\tau-\beta)(\omega b^\dagger b - g(b^\dagger+b))}e^{-\tau\omega b^\dagger b}|m\rangle + e^{\beta(\mu-v)}e^{\tau(\mu-U-v)}\langle m|e^{(\tau-\beta)\omega b^\dagger b}e^{-\tau(\omega b^\dagger b + g(b^\dagger+b))}|m\rangle\right], \end{aligned}$$

where $\alpha$ is a sum over the electronic states, and the Hamiltonian on the Matsubara branch is $H^M = H - \mu N$. To calculate this expression, we need to evaluate matrix elements of the general form

$$M = \langle m| e^{(\tau-\beta)(\omega b^\dagger b + f(b^\dagger+b))} e^{-\tau(\omega b^\dagger b + f'(b^\dagger+b))} |m\rangle. \tag{25}$$

This is efficiently done by noting that, since we trace over a complete set of phonon states, we can choose these states as eigenstates of a shifted harmonic oscillator that satisfy $(\omega b^\dagger b + f(b^\dagger + b))|m, f\rangle = (\omega m - f^2/\omega)|m, f\rangle$. These states are related to the unshifted harmonic oscillator states by $|m, f\rangle = \Lambda(f/\omega)|m\rangle$, with the translation operator $\Lambda(f/\omega) = e^{f/\omega(b^\dagger - b)}$ (this follows from a simplified version of the Lang-Firsov transformation). The matrix element $M$ can now be written as

$$\begin{aligned} M &= e^{(\tau-\beta)(\omega m - f^2/\omega)} \sum_k \langle m, f| e^{-\tau(\omega b^\dagger b + f'(b^\dagger+b))} |k, f'\rangle\langle k, f'|m, f\rangle \\ &= e^{(\tau-\beta)(\omega m - f^2/\omega)} \sum_k e^{-\tau(\omega k - f'^2/\omega)} |\langle k, f'|m, f\rangle|^2, \end{aligned}$$

where we have inserted a complete set of states $|k, f'\rangle$. What remains is the calculation of the overlap between shifted harmonic oscillator states. This was done e.g by Cahill and Glauber [4], who found

$$|\langle k, f'|m, f\rangle|^2 = \frac{k!}{m!}\left(\frac{f+f'}{\omega}\right)^{2(m-k)} e^{-(f+f')^2/\omega^2}\left[L_m^{(k-m)}\left(\frac{(f+f')^2}{\omega^2}\right)\right]^2 \quad \text{if} \quad k \le m, \tag{26}$$

$$|\langle k, f'|m, f\rangle|^2 = \frac{m!}{k!}\left(\frac{f+f'}{\omega}\right)^{2(k-m)} e^{-(f+f')^2/\omega^2}\left[L_k^{(m-k)}\left(\frac{(f+f')^2}{\omega^2}\right)\right]^2 \quad \text{if} \quad k \ge m, \tag{27}$$

where $L_n^{(\alpha)}$ is an associated Laguerre polynomial. For the case considered here, we always have $f + f' = \pm g$, so that the overlaps can be expressed more compactly as $|\langle k, f'|m, f\rangle|^2 = e^{-g^2/\omega^2} F_{mk}(g^2/\omega^2)$, where the function $F_{mk}$ is given by

$$F_{mk}(x) = \frac{k!}{m!} x^{(m-k)} \left[L_m^{(k-m)}(x)\right]^2 \quad \text{if} \quad k \le m, \tag{28}$$

$$F_{mk}(x) = \frac{m!}{k!} x^{(k-m)} \left[L_k^{(m-k)}(x)\right]^2 \quad \text{if} \quad k \ge m. \tag{29}$$

This gives the final expression for the $\tau > 0$ part of $G^M$ as

$$\begin{aligned} G^M(\tau) = & 2\sum_{mk} e^{-\beta(\omega m - g^2/\omega)} e^{-\tau(\omega(k-m)+v-\mu-g^2/\omega)} e^{-g^2/\omega^2} F_{mk}\left(\frac{g^2}{\omega^2}\right) \\ & + 2\sum_{mk} e^{-\beta(\omega m + v - \mu)} e^{-\tau(\omega(k-m)+U+v-\mu+g^2/\omega)} e^{-g^2/\omega^2} F_{mk}\left(\frac{g^2}{\omega^2}\right). \end{aligned} \tag{30}$$

Having evaluated $G^M(\tau)$, we can transform to energy using $G^M(i\omega_n) = \int dt e^{i\omega_n \tau} G^M(\tau)$, where $\omega_n = (2n+1)\pi/\beta$. This gives

$$\begin{aligned} G^M(i\omega_n) = & 2\sum_{mk} e^{-\beta(\omega m - g^2/\omega)} \frac{e^{-\beta(\omega(k-m)+v-\mu-g^2/\omega)} + 1}{i\omega_n - \omega(k-m) - v + \mu + g^2/\omega} e^{-g^2/\omega^2} F_{mk}\left(\frac{g^2}{\omega^2}\right) \\ & + 2\sum_{mk} e^{-\beta(\omega m + v - \mu)} \frac{e^{-\beta(\omega(k-m)+U+v-\mu+g^2/\omega)} + 1}{i\omega_n - \omega(k-m) - U - v + \mu - g^2/\omega} e^{-g^2/\omega^2} F_{mk}\left(\frac{g^2}{\omega^2}\right). \end{aligned} \tag{31}$$

To get the lesser and greater components of the spectral function we first perform the analytic continuation to real energies, $G^{R/A}(\epsilon) = G^M(\epsilon - \mu \pm i\delta)$, where $\delta$ is a positive infinitesimal, and then use the fluctuation-dissipation theorem

$$G^<(\epsilon) = -f(\epsilon - \mu)[G^R(\epsilon) - G^A(\epsilon)], \tag{32}$$

$$G^>(\epsilon) = \bar{f}(\epsilon - \mu)[G^R(\epsilon) - G^A(\epsilon)], \tag{33}$$

where $f$ is the Fermi-Dirac distribution and $\bar{f} = 1 - f$. Putting these expressions together, we find the greater part of the spectral function to be

$$A^>(\epsilon) = \frac{e^{-g^2/\omega^2}}{Z} \sum_{mk} F_{mk}\left(\frac{g^2}{\omega^2}\right) \times \\ \left[e^{-\beta(\omega m - g^2/\omega)}\delta(\epsilon - \omega(k-m) - v + g^2/\omega) + e^{-\beta(\omega m + v - \mu)}\delta(\epsilon - \omega(k-m) - U - v - g^2/\omega)\right],$$

where the partition function is given by $Z = (1-e^{-\beta\omega})^{-1}[e^{\beta g^2/\omega} + 2e^{\beta(\mu - v)} + e^{\beta g^2/\omega}e^{\beta(2\mu - U - 2v)}]$. To obtain this expression we have used that the function $\bar{f}$ cancels the numerator coming from the integration over $\tau$, when evaluated at the energy given by the delta function. Similarly, the lesser part of the spectral function is

$$A^<(\epsilon) = \frac{e^{-g^2/\omega^2}}{Z} \sum_{mk} F_{mk}\left(\frac{g^2}{\omega^2}\right) \times \\ \left[e^{-\beta(\omega k + v - \mu)}\delta(\epsilon - \omega(k-m) - v + g^2/\omega) + e^{-\beta(\omega k + U + 2v - 2\mu - g^2/\omega)}\delta(\epsilon - \omega(k-m) - U - v - g^2/\omega)\right],$$

where again we have simplified the expression using the cancellation due to the Fermi function. These expressions have the general structure of a sum of peaks at the addition (removal) energies of the system, weighted by the thermal occupation of the initial state and an overlap of quasi-particle amplitudes.

As a consistency check we note that in the limit $\beta \to \infty$, this formula should reproduce the zero temperature expression obtained by Langreth [5]. To obtain his expression we need to start from the state $|\uparrow, 0\rangle$ with one electron and zero phonons, instead of taking the trace over all states. This amounts to taking $m = 0$ in the expression above, and neglecting the two last terms that come from the initial state $|\uparrow\downarrow, 0\rangle$. In this limit the partition function becomes $Z = e^{\beta g^2/\omega}/(1 - e^{-\beta\omega})$, and we find

$$\begin{aligned} A^>(\epsilon) &= \frac{e^{-g^2/\omega^2}}{Z} \sum_k F_{0k}\left(\frac{g^2}{\omega^2}\right) e^{\beta g^2/\omega}\delta(\epsilon - \omega k - v + g^2/\omega) \\ &= e^{-g^2/\omega^2} \sum_k \frac{1}{k!}\left(\frac{g^2}{\omega^2}\right)^k \delta(\epsilon - \omega k - v + g^2/\omega), \end{aligned} \tag{34}$$

where in the first line we have used that $F_{0k}(x) = 1$ for all $k$. As expected, this gives the known zero temperature expression for $A^<$.

## DOUBLE OCCUPANCY

To gain some insights into the interplay of e-e and e-ph interactions, it is useful to look at the double occupancy $\mathcal{D} \equiv \langle n_\uparrow n_\downarrow\rangle = -\frac{1}{\beta}\partial_U \ln Z$. For the single-site system, this quantity can be obtained as an explicit function of the electron density $n$. This is done by noting that $\mathcal{D}/n = [2 + 2e^{\beta(U+v-\mu)}]^{-1}$, and that using the expression for $v$ given in the main text, we have $e^{\beta(U+v-\mu)} = (1-\delta n)/(\delta n + R)$ with $R = \sqrt{\delta n^2 + e^{-\beta U}(1-\delta n^2)}$. The exact DFT expression for the single-site system is therefore

$$\mathcal{D}^{ss}_{DFT}(\beta, n, U) = \left(\frac{1+\delta n}{2}\right)\frac{\delta n + \sqrt{\delta n^2 + e^{-\beta U}(1-\delta n^2)}}{1 + \sqrt{\delta n^2 + e^{-\beta U}(1-\delta n^2)}}. \tag{35}$$

In Fig. 2, we show $\langle n_\uparrow n_\downarrow\rangle$ for a 7-site chain with a HH impurity in the center. The exact $\mathcal{D}$ at the impurity is compared to $\mathcal{D}^{ss}_{DFT}$, which lacks kinetic energy effects, but has the exact $n$ as input and a $\beta$-value optimized for best agreement. We see that for small $\beta$ the DFT is in close agreement with the exact results, indicating that in some cases trading between kinetic and thermal effects can produce a nice agreement.

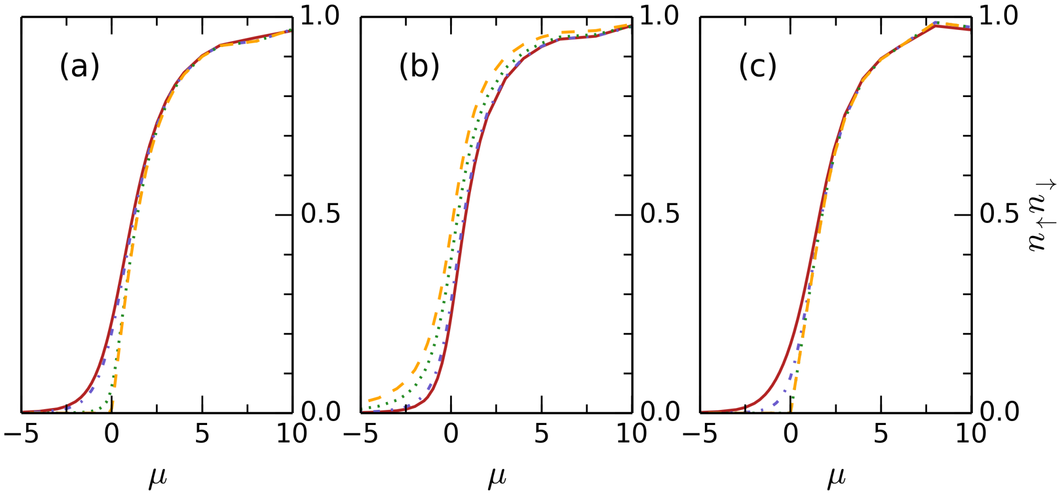


FIG. 2: Double occupancy $\mathcal{D} \equiv \langle n_\uparrow n_\downarrow \rangle$ at the impurity site as a function of the chemical potential $\mu$ for a 7-site chain with a Hubbard-Holstein impurity at the central site. In panel (a) $U = 1$ and $g = 1/4$, in panel (b) $U = 1$ and $g = 3/4$, while in panel (c) $U = 4$ and $g = 1$. In all cases, we take $v = -U/2$. The red curve represents the exact result for $\beta = \infty$, while the DFT results, obtained with $\mathcal{D}^{ss}_{DFT}$, are for $\beta = 1$ (violet), $\beta = 5$ (green), and $\beta = 10$ (yellow).

## DYNAMICS OF THE BETHE CHAIN

In this section we provide some further details on the dynamics of the chain system studied in the main text, governed by the Hamiltonian

$$H_{\text{chain}} = -J \sum_{i=0,\sigma}^{\infty} c^\dagger_{i\sigma} c_{i+1,\sigma} + \text{H.c.} + v(t)\hat{n}_0 + U\hat{n}_{0\uparrow}\hat{n}_{0\downarrow} + \omega b^\dagger b + g\hat{n}_0(b^\dagger + b). \tag{36}$$

As mentioned in the main text, the dynamics of the interacting site (labelled 0) exactly reproduces that of an infinitely coordinated Bethe lattice with a single interacting site in the center. To study the dynamics of this system we use a time-dependent extension of the density functional theory (DFT) formalism developed in the sections above. The time-dependent Kohn-Sham equations corresponding to Eqs. (13) and (14) above are given by

$$i\partial_t |\psi_m\rangle = \hat{H}^e(t)|\psi_m\rangle = \left[ -t \sum_{\langle ij\rangle\sigma} \left( \hat{c}^\dagger_{i\sigma}\hat{c}_{j\sigma} + h.c \right) + \sum_{i\sigma} v^{KS}_i[n,x](t)\hat{n}_{i\sigma} \right] |\psi_m\rangle \tag{37}$$

$$i\partial_t |\chi_n\rangle = \hat{H}^{ph}(t)|\chi_n\rangle = \sum_j \left[ \omega \hat{b}^\dagger_j \hat{b}_j + \sqrt{2}\eta_{KS}[n,x](t)\hat{x}_j \right] |\chi_n\rangle . \tag{38}$$

where the occupied single KS electron orbitals are added up to give the electronic density: $n(i,t) = \sum_m^{occ} |\langle i|\psi_m(t)\rangle|^2$. To solve these equations we use the adiabatic local density approximation, and take $\eta = 0$, which gives $v^{KS}_i[n,x](t) \approx v^{KS}_i(n_i(t), x_i(t))$ and $\eta^{KS}_j[n,x](t) \approx \eta^{KS}_j(n_j(t), x_j(t)) = g(n_j(t) - 1)$. Within this approximation, and specializing to the chain Hamiltonian, the Kohn-Sham equations simplify to

$$i\partial_t |\psi_m\rangle = \left[ -t \sum_{\langle ij\rangle\sigma} \left( \hat{c}^\dagger_{i\sigma}\hat{c}_{j\sigma} + h.c \right) + \left( v(t) + \frac{U}{2} n_0(t) + \sqrt{2} g x_0(t) + v_{xc}(n_0(t), x_0(t)) \right) \hat{n}_0 \right] |\psi_m\rangle \tag{39}$$

$$i\partial_t |\chi_n\rangle = \left[ \sum_j \omega \hat{b}^\dagger_j \hat{b}_j + \sqrt{2} g (n_0(t) - 1)\hat{x}_0 \right] |\chi_n\rangle . \tag{40}$$

We now consider a finite chain of length $L = 8$, corresponding to a Bethe lattice of 8 layers. The dynamics is performed using both exact diagonalization as well as TDDFT via the Kohn-Sham equations above. The potential

$v_{xc}$ is taken either from the DMFT solution discussed above, or from the analytic solution of a single HH site as given in the main text. By setting $v_{xc}$ to zero, we also consider the Hartree-Fock (HF) time evolution.

In Figure 3 we show the dynamics of the phonon coordinate $x_0$, corresponding to the electron density of Fig. 3 in the main text. In panels (a)-(c) we study a sudden interaction quench $(U_i, g_i) \to (U_f, g_f)$ at $t = 0$. For the quench $(0,0) \to (3,1)$ shown in panel (a) of Fig. 3, the exact and TDDFT-DMFT results are in excellent agreement, while the single-site potential and the HF solution give a moderately good description. Instead, for $(8,1) \to (3,1)$ and $(3,1) \to (8,1)$ as shown in panels (b) and (c), the agreement worsens due to stronger interactions. However, the DMFT potential still qualitatively performs well, while the HF solution fails to capture the main features.

Panels 3(d)-(f) show the dynamics induced by an external field $v(t)$ applied at the impurity site. In panel (d), where $U = 8$ and $g = 0.2$, $v(t)$ is ramped on in a time $T = 8$, and kept constant afterwards. Explicitly, we have

$$v(t) = \begin{cases} 0 & t \leq 0 \\ A \sin^2\left(\frac{\pi t}{2T}\right) & 0 \leq t \leq T \\ A & t \geq T \end{cases} \tag{41}$$

with $A = 1$ and $T = 8$. In this case there is excellent agreement between exact and TDDFT results. In panels (e) and (f), the potential $v(t)$ is a smoothed square pulse of duration $T = 4$, given by

$$v(t) = \begin{cases} A \sin^2\left(\frac{\pi t}{2T}\right) & 0 \leq t \leq T_1 \\ 1 & T_1 \leq t \leq T_1 + T_2 \\ A\left[1 - \sin^2\left(\frac{\pi(t-T_2)}{2T}\right)\right] & T_1 + T_2 \leq t \leq 2T_1 + T_2 \\ 0 & t \geq 2T_1 + T_2 \end{cases}, \tag{42}$$

with $A = 1$, $T_1 = 8$ and $T_2 = 4$. In (e), where $U = 8$ and $g = 1$, the DMFT potential gives a good agreement, while the single-site potential is slightly worse. In both cases, there is no trace of the artificial oscillation seen in the electron density when the density reaches half filling. In panel (f) we consider $U' < 0$, using only the single-site potential since the DMFT calculation have so far been restricted to $U' > 0$. We see that the single-site potential gives a very good agreement with the exact results.

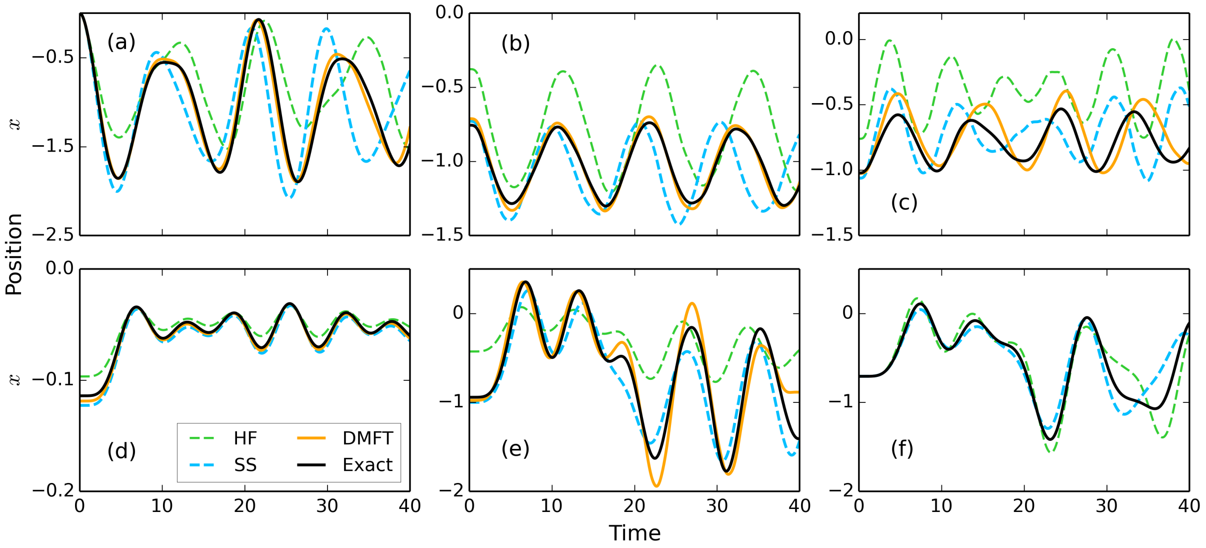


FIG. 3: Dynamics of an 8-site Anderson-Holstein chain with $n_\downarrow = n_\uparrow = 3$, for $J = 1$, $\omega = 1$, and $Z \to \infty$. In all panels, the optimization of $\beta$ gives a value $\beta \simeq 5$. Panels (a)-(c) correspond to a sudden quench of the interaction pair $(U, g)$; from left to right, $(0,0) \to (3,1), (8,1) \to (3,1)$, and $(3,1) \to (8,1)$, respectively. In panel (d), $U = 8$ and $g = 0.2$ and the external potential is ramped to $v = 1$ in a time $T = 8$. For panels (e) and (f) the interactions are $U = 8$ and $g = 1$ or $U = 1$ and $g = 0.5$ respectively, and the external field is a pulse of strength $v = 1$ and duration $T = 4$.

[1] M. Levý, PNAS **76** (12), 6062-6065 (1979).
[2] K. Schönhammer, O. Gunnarsson, and R. M. Noack, Phys. Rev. B **52**, 2504 (1995).
[3] C.-O. Almbladh (private communication).
[4] K. E. Cahill and R. J. Glauber, Phys. Rev. **177**, 1857 (1969).
[5] D. Langreth, Phys. Rev. B **1**, 471 (1970).
[6] P. Werner, A. Comanac, L. de' Medici, M. Troyer, and A. J. Millis, Phys. Rev. Lett. **97**, 076405 (2006).
[7] P. Werner and A. J. Millis, Phys. Rev. Lett. **99**, 146404 (2007).
[8] M. Farzanehpour, I. V. Tokatly, Phys. Rev. B **90**, 195149 (2014).
